# Supplementary material for: A Parameterized Perspective on Protecting Elections
Source: arXiv:1905.11838 source file (2019-05-28)
Supplement: Supplementary file 1 [file appendix.tex]

\section*{Appendix}

\begin{theorem}
 The $k$-{\sc Sum} problem is \NPC.
\end{theorem}

\begin{proof}
 
\end{proof}
